# Supplementary material for: Taming the War in Memory: A Resilient Mitigation Strategy Against Memory Safety Attacks in CPS
Source: arXiv:1809.07477 source file (2019-09-19)
Supplement: Supplementary file 1 [file 11_appendix.tex]

\appendix
%\begin{appendices}
\section{Appendix}

%\begin{figure}[thb]
%%\parbox[t]{7cm}{\null
%  \centering
%  %\rule{3cm}{3cm}%
%  %\includegraphics[width=0.4\textwidth,height=0.4\textheight]{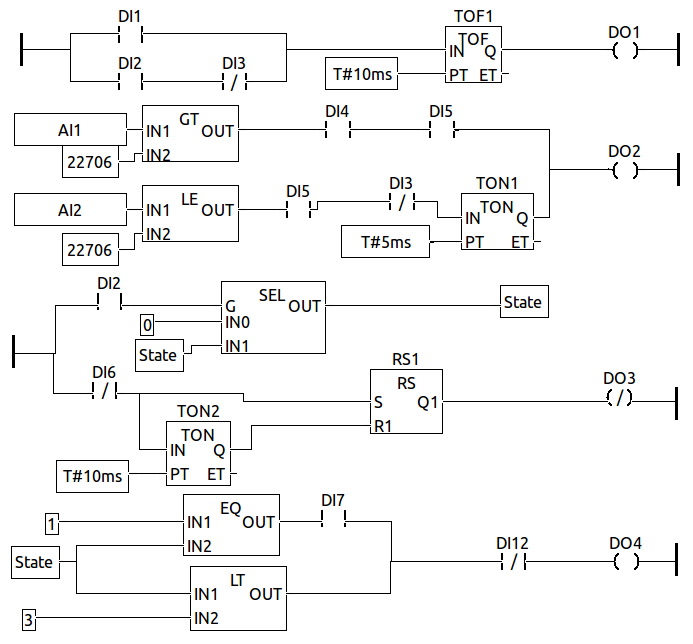} 
%  \includegraphics[scale=0.36]{images/plc_program}
%  \caption{Sample PLC program in ladder diagram}
%  \label{fig:logic_diagram}
%%}
%\end{figure}

\begin{figure}[htb]	
%-attacks\vspace{-20pt}
	\centering
        \includegraphics[scale=0.43]{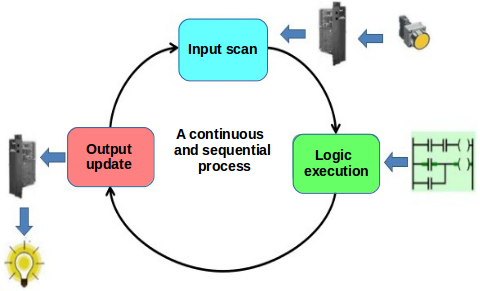}
  		\captionof{figure}{The scan cycle of a PLC}
  		\label{fig:scan_cycle}
\end{figure}

%\parbox[t]{7cm}{\null

  %\vskip-\abovecaptionskip
  %\captionof{table}[t]{Instruction count}
\REM{  \begin{table}[htb]\label{table:program_complexity}
  \centering
 % \vskip\abovecaptionskip
  %\begin{tabular}{cc} \hline
\caption{Instruction count}
\label{table:instruction_count}
%\scalebox{0.75}{
 \begin{tabular}{|l|c|}
\hline
Instructions                                                                      & Count                                         \\ \hline
\begin{tabular}[c]{@{}l@{}}Logical\\ \quad AND\\ \quad OR\\ \quad NOT\\ \quad SR\end{tabular}                  & \begin{tabular}[c]{@{}l@{}}\\ 17\\ 14\\ 5\\ 1\end{tabular}           \\ \hline
\begin{tabular}[c]{@{}l@{}}Arithmetic\\ \quad ADD\\ \quad MUL\end{tabular}  & \begin{tabular}[c]{@{}l@{}}\\ 1\\ 2\end{tabular}     \\ \hline
\begin{tabular}[c]{@{}l@{}}Comparisons\\ \quad EQ\\ \quad GT\\ \quad LT\\ \quad LE\end{tabular} & \begin{tabular}[c]{@{}l@{}}\\ 3\\ 3\\ 2\\ 2\end{tabular} \\ \hline
\begin{tabular}[c]{@{}l@{}}Timers\\ \quad TON\\ \quad TOF\end{tabular}                        & \begin{tabular}[c]{@{}l@{}}\\ 3\\ 9\end{tabular}                \\ \hline
\begin{tabular}[c]{@{}l@{}}Counters\\ \quad CTU\end{tabular}                      & \begin{tabular}[c]{@{}l@{}}\\ 1\end{tabular}                 \\ \hline
\begin{tabular}[c]{@{}l@{}}Selections\\ \quad SEL\\ \quad MAX\end{tabular}            & \begin{tabular}[c]{@{}l@{}}\\1\\ 1\end{tabular}             \\ \hline
\begin{tabular}[c]{@{}l@{}}Contacts\\ \quad NO\\ \quad NC\end{tabular}                        & \begin{tabular}[c]{@{}l@{}}\\ 38\\ 3\end{tabular}                \\ \hline
\begin{tabular}[c]{@{}l@{}}Coils\\ \quad NO\\ \quad NC\end{tabular}                           & \begin{tabular}[c]{@{}l@{}}\\ 21\\ 2\end{tabular}                \\ \hline
Total                                                                             & 129                                                           \\ \hline
\end{tabular}
\end{table}
}
